# Supplementary material for: Media Bias Detector: Designing and Implementing a Tool for Real-Time Selection and Framing Bias Analysis in News Coverage
Source: arXiv:2502.06009 source file (2025-04-28)
Supplement: Supplementary file 1 [file website_methodology_appendix.pdf]

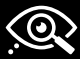

## Methodology

The initial focus of the Media Bias Detector is to showcase real-time dashboards of what we deemed most important and tractable about what is being produced in the news this week.

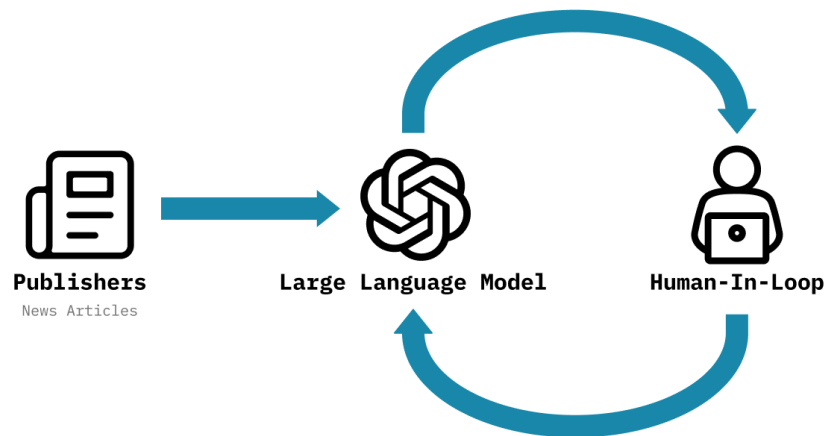

Figure 1 shows a schematic of our data pipeline, which we describe in detail below.

## Project Glossary

▼ View Table

| Term       | Definition                                                                                                                                                                                                                                                         | Note                   |
|------------|--------------------------------------------------------------------------------------------------------------------------------------------------------------------------------------------------------------------------------------------------------------------|------------------------|
| Bias       | Preferential selection of stories, facts, people, events, or viewpoints.                                                                                                                                                                                           |                        |
| Cluster    | A group of articles or sentences that are talking about the same issue.                                                                                                                                                                                            |                        |
| Absorption | "Absorption" is defined by respondents in a survey either noting they recall a topic from the previous week or including a fact, opinion, or narrative in open answers about the news.                                                                             | Dataset: Tracking_Poll |
| Event      | An event is an incident that happens in the world which is substantial enough that a considerable number of articles are written on it in a short period of time. Events are detected algorithmically defined based on clusters of articles on a three-day window. |                        |
| Fact       | "Fact" is a statement that could in principle be known or proved to be true based on evidence. Importantly, we don't actually verify facts so they may or may not be true.                                                                                         | Dataset: Fact          |
| Opinion    | "Opinion" is a statement that expresses the subjective view or interpretation of the author                                                                                                                                                                        | Dataset: Fact          |

| Term  | Definition                                                                                                                                                                                                                                                                                                                                                                                                                                                                                                                                                                                                                                                                                                        | Note          |
|-------|-------------------------------------------------------------------------------------------------------------------------------------------------------------------------------------------------------------------------------------------------------------------------------------------------------------------------------------------------------------------------------------------------------------------------------------------------------------------------------------------------------------------------------------------------------------------------------------------------------------------------------------------------------------------------------------------------------------------|---------------|
|       | about some topic; it is not necessarily based on fact or knowledge.                                                                                                                                                                                                                                                                                                                                                                                                                                                                                                                                                                                                                                               |               |
| Lean  | The extent to which the article either explicitly or implicitly aligns with the viewpoints, policies, or concerns of Republicans vs. Democrats. Lean does not necessarily imply that the article is “pro” one party or the other. It may simply be that the topic of the article is inherently of more interest to Democrats or Republicans. For example, GPT tends to code stories about reproductive rights issues as “D” on the grounds that it believes democratic voters tend to share these concerns more than republican voters. The articles themselves need not mention either party or advocate for either party’s policies. See <a href="#">here</a> for more details on how GPT codes articles’ lean. | Dataset: Fact |
| Tone  | The extent to which the article overall has a positive vs. negative tone, as understood by GPT.                                                                                                                                                                                                                                                                                                                                                                                                                                                                                                                                                                                                                   | Dataset: Fact |
| Theme | A summary of the titles in an event cluster.                                                                                                                                                                                                                                                                                                                                                                                                                                                                                                                                                                                                                                                                      |               |

## Data Collection

Initially, we aim to analyze 10 online newspapers: Associated Press News, Breitbart News, CNN, Fox News, The Guardian, The Huffington Post, The New York Times, USA Today, The Wall Street Journal, and The Washington Post. We chose these publications for their mix of reach and agenda-setting influence, where we plan to add more publications going forward.

We look at each publisher’s homepage five times daily, at 6 AM, 10 AM, 2 PM, 6 PM, and 10 PM EST. Then, we use article placement on the homepage to identify the top 20 most prominent articles displayed to readers. We assign position on the page as a combination of: distance from the top, size of the font, and inclusion and size of figures. Currently, we disregard content that does not focus on text, such as videos, podcasts, and photo galleries.

Next, we recover the article text, title, and date of publication. We preprocess the text beforehand to ensure superfluous text is not passed into the large language model. We remove advertisements, direct mentions of the publisher outside the context of the story, and repetitive phrases that are irrelevant to the article (e.g. “Listen 5 minutes”, “Click Here for More Information”, “Enter your email address”). We are continuing to grow this dictionary of boilerplate phrases as we collect more data.

## Classification

Next, we use GPT to generate labels for each document. The labels are generated at two levels: the article level and the sentence level. For simpler tasks, such as determining the topic, we employ GPT-3.5 Turbo, while for more complex tasks, we use GPT-4o. In the following sections, we summarize the list of extracted features and provide the exact prompts used for each task.

## Articles

**Takeaways:** 3-4 sentences that summarize the article.

▼ View code (model: GPT-3.5-turbo)

```
'''
The following is a news article. Read it and perform the task that follows.
Respond with a JSON object of key-value pairs.

#####

{article}

#####

Task: Summarize the main points of the news article.

Instruction: List short takeaway points that readers are likely to remember
from the article.
Key: "takeaways"
Value: A 3-4 sentence summary in a JSON list format.
'''
```

**Category/Topic/Subtopic:** We classify each article into a hierarchy of topics/subtopics. We predefine a master topic hierarchy and ask GPT to select topics from this list. Currently, the list contains 36 topics across eight categories: Politics, Culture and Lifestyle, Business, Health, Disaster, Economy, Sports, and Science and Technology. Each predefined topic is mapped to one of these eight categories, defaulting to Politics when an article may fall in several categories. To ensure that labeling subtopics remains tractable, GPT is presented with a set of predefined subtopics based on the topic that it initially selects.

[Here is the list](#) of categories, topics, and subtopics.

▼ View code (model: GPT-4o)

```
'''
The following is a news article. Read it and perform the task that follows.
Respond with a JSON object of key-value pairs.

#####

{article}
```

```
#####
```

Task: Classify the article into one of the listed topics.

Instruction: Try your best to bucket the article into one of these topics. DO NOT write anything that is not listed.

Key: "topic"

Value: One of: {topic\_list}.

Do not return anything except the JSON object of key-value pairs as output.  
'''

'''  
The following is a news article on the topic of {predicted\_topic}. Read it and perform the task that follows. Respond with a JSON object of key-value pairs.

```
#####
```

{article}

```
#####
```

Task: Classify the article into one of the listed subtopics under the predicted topic.

Instruction: Try your best to bucket the article into one of these subtopics. Label it as 'Other' if the article does not fit any possible subtopics.

Key: "subtopic"

Value: One of: {subtopic\_list\_under\_the\_topic}.

Do not return anything except the JSON object of key-value pairs as output.  
'''

**News type:** Each article's type is assigned to one of news report, news analysis, or opinion piece.

▼ View code (model: GPT-4o)

'''  
The following is a news article. Read it and perform the task that follows. Respond with a JSON object of key-value pairs.

```
#####
```

{article}

```
#####
```

Task: Determine the news type of this news article.

1. Instruction: Classify the above news article into one of three categories: news report, news analysis, or opinion. Each category has distinct characteristics:

- News Report: Objective reporting on recent events, focusing on verified facts without the writer's personal views.
- News Analysis: In-depth examination and interpretation of news events, providing context and explaining significance, while maintaining a degree of objectivity.
- Opinion: Articles reflecting personal views, arguments, or beliefs on current issues, often persuasive and subjective.

Consider criteria such as language objectivity, focus on facts versus interpretation, author's intent, and article structure.

Key: "news\_type"

Value: One of "news report" or "news analysis" or "opinion".

2. Instruction: Provide a short paragraph to justify your classification, citing specific elements from the text.

Key: "justification"

Value: A paragraph of text.

Do not return anything except the JSON object of key-value pairs as output.  
'''

**Article Tone:** Tone of the article is what GPT detects as the tone and no further description is provided. Tone of the article is elicited on a [-5, 5] scale, and then we bucket the results into five categories of “Very negative” [-5,-4], “Negative” [-3,-2], “Neutral” [-1,0,1], “Positive” [2,3], and “Very Positive” [4,5].

We label the article’s text and title separately for their tone.

▼ View code (model: GPT-4o)

'''

The following is a news article. Read it and perform the task that follows.  
Respond with a JSON object of key-value pairs.

#####

{article}

#####

Task: Determine the overall tone of the article. Is it negative, positive, or neutral?

1. Instruction: Provide a short paragraph summarizing in what ways the article has a negative or positive tone.

Key: "reason"

Value: A paragraph of text.

2. Instruction: Provide a number from -5 to 5, with -5 indicating a very negative tone and 5 indicating a very positive tone. A value of 0 indicates

```

that the article has a neutral tone.
  Key: "tone"
  Value: An integer number from -5 to 5.

Do not return anything except the JSON object of key-value pairs as output.
'''

'''
The following is the title of a news article on the topic of {topic}
({subtopic}) in the {category} news category. Read it and perform the task
that follows. Respond with a JSON object of key-value pairs.

#####

{title}

#####

Task: Determine the overall tone of the article title. Is it negative,
positive, or neutral?

1. Instruction: Provide a short paragraph summarizing in what ways the article
title has a negative or positive tone.
  Key: "reason"
  Value: A paragraph of text.

2. Instruction: Provide a number from -5 to 5, with -5 indicating a very
negative tone and 5 indicating a very positive tone. A value of 0 indicates
that the article title has a neutral tone.
  Key: "tone"
  Value: An integer number from -5 to 5.

Do not return anything except the JSON object of key-value pairs as output.
'''

```

**Article Political Lean:** The political lean is defined as the extent to which the article supports viewpoints, politicians, and/or policies of one party or the other in the context of U.S. politics. The lean of the article is elicited on a [-5, 5] scale, and then bucketed into five categories: “Democratic” [-5,-4], “Neutral Leaning Democratic” [-3,-2], “Neutral” [-1,0,1], “Neutral Leaning Republican” [2,3], and “Republican” [4,5]. We label the article’s text and title separately for their political lean. [Read more details on how GPT codes lean.](#)

▼ View code (model: GPT-4o)

```

'''
The following is a news article. Read it and perform the task that follows.
Respond with a JSON object of key-value pairs.

#####

{article}

```

#####

Task: Determine the political leaning of this article within the U.S. political context. Is it supporting the Democrat party or the Republican party? Supporting a party can mean supporting its viewpoints, politicians, or policies. Provide reasoning for your answer.

1. Instruction: Give a short paragraph summarizing in what ways the article supports the Democrat party or the Republican party.

Key: "reason"

Value: A paragraph of text.

2. Instruction: Give a number from -5 to 5, with -5 indicating strong support for Democrats and 5 indicating strong support for Republicans. A value of 0 indicates that the article has no clear political leaning towards either side.

Key: "lean"

Value: An integer number from -5 to 5.

Do not return anything except the JSON object of key-value pairs as output.

'''

'''

The following is the title of a news article on the topic of {topic} ({subtopic}) in the {category} news category. Read it and perform the task that follows. Respond with a JSON object of key-value pairs.

#####

{title}

#####

Task: Determine the political leaning of this article title within the U.S. political context. Is it supporting the Democrat party or the Republican party? Supporting a party can mean supporting its viewpoints, politicians, or policies. Provide reasoning for your answer.

1. Instruction: Provide a short paragraph summarizing in what ways the article title supports the Democrat party or the Republican party.

Key: "reason"

Value: A paragraph of text.

2. Instruction: Provide a number from -5 to 5, with -5 indicating strong support for Democrats and 5 indicating strong support for Republicans. A value of 0 indicates that the article title has no clear political leaning towards either side.

Key: "lean"

Value: An integer number from -5 to 5.

Do not return anything except the JSON object of key-value pairs as output.

'''

## Sentences

We also elicit sentence level labels for certain features, including sentence type, tone, and focus. The sentence type labels are used to extract facts in the event clustering step described later, and the tone and focus are used to investigate their correlation with the article tone and lean labels.

**Sentence type:** The type of sentence is one of "fact", "opinion", "borderline", "quote", or "other". A "fact" is something that's capable of being proved or disproved by objective evidence. An "opinion" reflects the beliefs and values of whoever expressed it, but should not be a quote. A "borderline" sentence is one that is not entirely a fact or opinion. A "quote" is a passage from another person or source that comes with quotation marks.

**Sentence tone:** Tone of each sentence is what GPT detects as the tone and no further description is provided. Sentence tone is one of “positive”, “negative”, or “neutral”.

**Sentence focus:** The focus measures whether the sentence is referring to one political party or the other.

▼ View code (model: GPT-4o)

```
"""
The following is a numbered list of sentences from a news article. Read them
all and perform the task that follows:

#####

{sentences}

#####

Task: For each sentence above, perform the following analysis. Return the
output as a list of JSON objects of key-value pairs, one for each sentence,
where the keys are:

1. Instruction: Output the number of the current sentence being analyzed.
Key: "sentence"
Value: The sentence number.

2. Instruction: Determine whether the sentence is a "fact", "opinion",
"borderline", "quote", or "other" type of sentence. A "fact" is something
that's capable of being proved or disproved by objective evidence. An
"opinion" reflects the beliefs and values of whoever expressed it, but should
not be a quote. A "borderline" sentence is one that is not entirely a fact or
opinion. A "quote" is a passage from another person or source that comes with
quotation marks. If a quote is composed of multiple sentences, they should all
be labeled as "quote".
Key: "type"
Value: One of "fact", "opinion", "borderline", "quote", "other". Select
"other" if the sentence does not fit the possible values.
```



```
3. Instruction: Classify the tone of the sentence as "positive", "negative",  
or "neutral".
```

```
Key: "tone"
```

```
Value: One of "positive", "negative", "neutral".
```

```
4. Instruction: Classify the focus of the sentence as being "democrat",  
"republican", or "neither" within the U.S. political context. If the sentence  
is referring to the Democratic Party, including its policies or politicians,  
label it as "democrat". If it is referring to the Republican Party, including  
its policies or politicians, label it as "republican". If it is referring to  
both, label it as "both". Otherwise, label it as "neither".
```

```
Key: "focus"
```

```
Value: One of "democrat", "republican", "both", "neither".
```

```
Do not return anything except the list of JSON objects of key-value pairs as  
output. Do not skip analyzing any sentences. Do not return any key values  
except those specified.
```

```
"""
```

## Events

To identify articles about the same event, we cluster them together based on their semantic similarity. We use GPT's large-context embedding model to obtain document embeddings for all articles and perform pairwise cosine similarity comparisons between all articles in a three-day sliding window. We then build a graph where nodes represent individual articles and edges represent the amount of similarity between them. By dropping edges below an empirically-determined threshold of 0.8, we are left with dense connected components which represent cohesive article clusters around news events. To make these clusters interpretable, we use GPT-4 to assign them thematic titles based on the titles of their constituent articles.

We extract the top facts around a particular event by tokenizing all articles within an event into sentences and keeping only those that have been labeled as factual statements by GPT. We then repeat the above embedding-based graph clustering process at the fact level with a threshold of 0.85. Oft-repeated facts appear as large clusters of highly similar statements, and we summarize each of these into a synthetic fact using GPT-4. These summary facts capture the most important pieces of information about a particular event and are used to study which facts publishers select to publish and which ones they leave out.

## Article cluster themes

▼ View code (model: GPT-4o)

```
"""
```

```
The following is a list of titles of a collection of news articles around a  
particular event. Read them and perform the task that follows. Respond with a  
JSON object of key-value pairs.
```

```
#####
```

```
{article_titles}
```

```
#####
```

Task: Summarize the titles.

1. Instruction: Analyze the titles and produce a good thematic title that best summarizes the event.

Key: "theme"

Value: The thematic title.

2. Instruction: Analyze the titles and produce a shorter title that is not longer than 4 to 5 words.

Key: "theme\_short"

Value: The shorter title.

Do not return anything except the JSON object of key-value pairs as output.

```
""
```

## Fact cluster themes

▼ View code (model: GPT-4o)

```
'''
```

The following is a list of sentences about the same event. Read them and perform the task that follows. Respond with a JSON object of key-value pairs.

```
#####
```

```
{sentence_list}
```

```
#####
```

Task: Analyze them and produce a comprehensive sentence that summarizes all of them and is no longer than 25 words.

Key: "synthetic\_sentence"

Value: The comprehensive sentence.

Do not return anything except the JSON object of key-value pairs as output.

```
'''
```

## Human-in-the-loop verification

We have hired a team of research assistants (RAs) to serve as "humans-in-the-loop." The RAs continually monitor a random sample of the labels generated by GPT to ensure that the model's accuracy remains high. They review topics, subtopics, and event clusters daily, and assess the remaining features on a weekly basis. At the end of each week, we re-evaluate the model's accuracy across all features and implement necessary

adjustments. If the accuracy falls below acceptable levels, we conduct a deep-dive into that category and adjust our prompting strategies.

### **Topic and subtopic verification:**

Each research assistant (RA) is presented with the key takeaways and the topic/subtopic generated by GPT for each article. They are then asked to verify if the generated topic accurately captures the article's content. If it does not, they provide an alternative topic/subtopic from our continuously updated [master list](#).

Sampling strategy: Balanced Sample with at least 10% of Articles per Topic

From yesterday's articles, ensure the sample includes at least 10% of articles from the topic category. If a topic has fewer than 10 articles, include at least one article from that topic. Balance the sample across different publishers to maintain diversity. Please include as many fields as possible.

### **Event and fact cluster verification:**

RAs review the top 10 event/fact clusters every day and determine whether each article/fact meaningfully belongs to the associated cluster or not.

Sampling Strategy: Top 10 Event Clusters from a 3-Day Window

Identify and sample the top 10 event clusters from articles published in the last three days. Select the top clusters sorted by the number of articles in the cluster.

### **Article and title lean/tone:**

For political leaning and tone, research assistants (RAs) are presented with the article's text and title separately and asked to provide their own evaluation of its political leaning and tone using the same five-point scale displayed on the dashboard for each metric. Unlike with topic/subtopic, the RAs are not provided with the GPT labels and are asked directly for their own judgment.

Sampling Strategy: Sample with 2 Articles per Lean/Tone Bucket

From yesterday's articles, select 2 articles from each article lean/tone bucket. Ensure that at least one article from each publisher is included in the sample, aiming for a total of 20 samples per day. Adjust this strategy as needed based on weekly reviews. Please include as many fields as possible.
